# Supplementary material for: Solving the Closest Vector Problem with respect to l_p Norms
Source: arXiv:1104.3720 source file (2011-09-26)
Supplement: Supplementary file 1 [file Appendix_ReplacementProcedure.tex]

\subsection{Description of the Replacement Procedure} \label{sec_appendix_replacement_procedure}

\noindent In this section, we present the decomposition procedure developed by Frank and Tardos, \cite{pp_ft87}.
The main tool for the decomposition algorithm is simultaneous diophantine approximation.\\
A famous result due to Dirichlet is that for all integers $N \in \mathbbm{N}$ and real numbers $\alpha_1, \hdots, \alpha_n \in \mathbbm{R}$, there exists $p_1, \hdots, p_n \in \mathbbm{z}$ and $q \in \mathbbm{Z}$ such that
$1 \leq q \leq N^n$ and
$| q \cdot \alpha_i - p_i | < 1 / N$
for all $1 \leq i \leq n$.\\
Unfortunately, Dirichlet's result is not constructive.
but using the LLL-algorithm such a simultaneous diophantine approximation for given rational numbers can be computed efficiently.\\

\begin{figure}[t]
\begin{center}
\framebox{
\begin{minipage}[b]{15.5cm} \small
\begin{alg} \label{alg_subroutine} {Replacement Procedure}\\
{\tt
{\bf Input:}
	A parameter $N \in \mathbbm{N}$,\\
	an affine subspace $\bigcap_{i=m+1}^n H_{k_i,d_i}$ and\\
	an additional hyperplane $H_{k,d}$, such that $d,d_{m+1}, \hdots, d_n$ are linearly independent.\\
{\bf Used Subroutine:} Decomposition algorithm
\begin{enumerate}
 \item Apply the decomposition algorithm to the $(n+1)$-dimensional vector $w = ( d^T , k )^T$ and the parameter $N \in \mathbbm{N}$.\\
 		We obtain vectors $( \bar{d}_i^T , \bar{k}_i )^T \in \mathbbm{Z}^{n+1}$, where $1 \leq i \leq j ( m ) \leq n + 1$, together with parameters $\chi_i$, $1 \leq i \leq j ( m )$.
 	\item Let $I \subseteq \{ 1 , \hdots, j ( m ) \}$ be the maximal set of indices such that the vectors $d_i$, $m+1 \leq i \leq n$ and $\bar{d}_i$, $i \in I$ are linearly independent.
\end{enumerate}
{\bf Output: } Hyperplanes $H_{\bar{k}_i,\bar{d}_i}$ with $i \in I$.
}
\end{alg}
\end{minipage}}
\end{center}
\end{figure}

\begin{prop} (Proposition \ref{prop_replacement_procedure} restated)\\
There exists a replacement proceudre, which satisfies the following properties:\\
Given as input a parameter $N \in \mathbbm{N}$, an affine subspace $H$ and an additional affine hyperplane $H_{k,d}$ the replacement procedure computes a set of hyperplanes $H_{\bar{k}_i, \bar{d}_i}$, $i \in I \not= \emptyset$, such that the following holds:
\begin{itemize}
	\item The representation size of the vectors $\bar{d}_i \in \mathbbm{Z}^n$ and the numbers $\bar{k}_i \in \mathbbm{Z}$ is at most
		$$2^{(n+1)(n+2)} N^n.$$
	\item Every vector $z \in B_n^{(1)} ( 0 , N-2 ) \cap H$ satisfies $\langle d , z \rangle = k$ if and only if it satisfies $\langle \bar{d}_i , z \rangle = \bar{k}_i$ for all $i \in I$.
	\item The number of arithmetic operations is at most ...
\end{itemize}
\end{prop}

\begin{proof}
First, we show that $I \not= \emptyset$.
The vector $(d^T,k)^T$ is a linear combination of the vectors $(\bar{d}_i^T,\bar{k}_i)^T$, $1 \leq i \leq j ( m )$.
Especially, $d$ is a linear combination of the vectors $\bar{d}_i$.\\
By assumption, the vectors $d_{m+1}, \hdots, d_n , d$ are linearly independent.
Hence, there exists at least one vector $\bar{d}_i$, $1 \leq i \leq j ( m )$, such that $d_{m+1}, \hdots, d_n , \bar{d}_i$ are linearly independent.\\
The upper bound on the representation size follows directly from Theorem \ref{}, since each vector computed by the decomposition algorithm is an integer vector with
$\| ( \bar{d}_i^T , \bar{k}_i )^T \|_{\infty} \leq 2^{(n+1)(n+2)} N^n$.\\
Since every vector in $z \in B_n^{(1)} ( 0 , N-2 )$ satisfies
$\| z \|_1 \leq N - 2$, the vector
$z' = ( z^T , -1 )^T \in \mathbbm{R}^{n+1}$ satisfies
$\| z' \|_1 = \| z \|_1 + 1 \leq N - 1$.
Hence, it follows from Lemma \ref{} that $z'$ is orthogonal to the vector $(d^T,k)^T$ if and only if it is orthogonal to the vector $(\bar{d}_i^T,\bar{k}_i)^T$, $1 \leq i \leq j (m )$, which provides a linear combination of it:
$\langle z' , ( d^T , k )^T \rangle = 0$ if and only if
$\langle z' , ( \bar{d}_i^T , \bar{k}_i^T ) \rangle = 0$ for all $1 \leq i \leq j ( m )$.\\
This means that the vector $z$ is contained in the hyperplane $H_{k,d}$ if and only if it is contained in the intersection of the hyperplanes $H_{\bar{k}_i, \bar{d}_i}$, $1 \leq i \leq j ( m )$
and it shows that $z \in B_n^{(1)} ( 0 , N-2 )$ is contained in $H \cap H_{k,d}$ if and only if it is contained in $H \cap \bigcap_{i=1}^{j(m)} H_{\bar{k}_i,\bar{d}_i}$.\\
The set $I$ is maximal with the property that the vectors $d_{m+1} , \hdots, d_n $ and $\bar{d}_i$, $i \in I$, are linearly independent.
Hence, a vector $z \in B_n^{(1)} ( 0 , N-2 )$ is contained in the affine subspace $H \cap H_{k,d}$ if and only if it is contained in the affine subspace $H \cap \bigcap_{i \in I} H_{\bar{k}_i,\bar{d}_i}$.
\end{proof}
